# Supplementary material for: Maximizing the minimum achievable secrecy rate of two-way relay networks using the null space beamforming method
Source: arXiv:1611.05839 source file (2016-11-17)
Supplement: Supplementary file 1 [file AppendixII.tex]

\textcolor[rgb]{0,0.5,0}{\section{APPENDIX II}}
\textcolor[rgb]{0,0.5,0}{In this section, the mathematical steps towards finding (\ref{botpage1}) and (\ref{botpage2}) will be discussed. To this end, the mutual information between ${{\mathbf{y}}_{{E}}}$ and ${x}_{2}$ can be computed as,}
\textcolor[rgb]{0,0.5,0}{\begin{equation}\label{AppII1}
\begin{aligned}
 &I\left( {{x}_{2}};{{\mathbf{y}}_{E}} \right)\,=\mathcal{H}\left( \,{{\mathbf{y}}_{E}} \right)-\mathcal{H}\left( \,{{\mathbf{y}}_{E}}|{{x}_{2}} \right)\,\\
 &\,\,\,\,\,\,\,\,\,\,\,\,\,\,\,\,\,\,\,~~~\,=\,{{\log }_{2}}\,\det \left( \text{ }\!\!\pi e\,{{\mathbf{K}}_{{{\mathbf{y}}_{E}}}} \right)-{{\log }_{2}}\,\det \left( \text{ }\!\!\pi e\,{{\mathbf{K}}_{{{\mathbf{y}}_{E}}|{{x}_{2}}}} \right) \\
 & \,\,\,\,\,\,\,\,\,\,\,\,\,\,\,\,\,\,\,~~~\,={{\log }_{2}}\frac{\det \left( {{\mathbf{K}}_{{{\mathbf{y}}_{E}}}} \right)}{\det \left( {{\mathbf{K}}_{{{\mathbf{y}}_{E}}|{{x}_{2}}}} \right)},
 \end{aligned}
\end{equation}}
\textcolor[rgb]{0,0.5,0}{where $\mathcal{H}(.)$ and $det(.)$ denote, respectively, the entropy and the determinant functions. In this case, the covariance matrices ${{\mathbf{K}}_{{{\mathbf{y}}_{E}}}}$ and ${{\mathbf{K}}_{{{\mathbf{y}}_{E}}|{{x}_{2}}}}$ can be computed as follows,}
\textcolor[rgb]{0,0.5,0}{\begin{equation}\label{AppII2}
  {{\mathbf{K}}_{{{\mathbf{y}}_{E}}}}=\,\text{E}\left\{ {{\mathbf{y}}_{E}}\mathbf{y}_{E}^{\text{H}} \right\}=\left[ \begin{matrix}
   {{\left| {{g}_{1}} \right|}^{2}}{{\text{P}}_{1}}+{{\left| {{g}_{2}} \right|}^{2}}{{\text{P}}_{2}}+\sigma _{E\text{,1}}^{2} & {{g}_{1}}{{\left( \mathbf{f}_{e}^{\text{T}}\mathbf{W}{{\mathbf{f}}_{1}} \right)}^{*}}{{\text{P}}_{1}}+{{g}_{2}}{{\left( \mathbf{f}_{e}^{\text{T}}\mathbf{W}{{\mathbf{f}}_{2}} \right)}^{*}}{{\text{P}}_{2}}  \\
   g_{1}^{*}\left( \mathbf{f}_{e}^{\text{T}}\mathbf{W}{{\mathbf{f}}_{1}} \right){{\text{P}}_{1}}+g_{2}^{*}\left( \mathbf{f}_{e}^{\text{T}}\mathbf{W}{{\mathbf{f}}_{2}} \right){{\text{P}}_{2}} & {{\left| \mathbf{f}_{e}^{\text{T}}\mathbf{W}{{\mathbf{f}}_{1}} \right|}^{2}}{{\text{P}}_{1}}+{{\left| \mathbf{f}_{e}^{\text{T}}\mathbf{W}{{\mathbf{f}}_{2}} \right|}^{2}}{{\text{P}}_{2}}+\sigma _{R}^{2}||\mathbf{f}_{e}^{\text{T}}\mathbf{W}|{{|}^{2}}+\sigma _{E\text{,2}}^{2}  \\
\end{matrix} \right],
\end{equation}}

\textcolor[rgb]{0,0.5,0}{\begin{equation}\label{AppII3}
   {{\mathbf{K}}_{{{\mathbf{y}}_{E}}|{{x}_{2}}}}=\,\text{E}\left\{ \left( {{\mathbf{y}}_{E}}|{{x}_{2}} \right){{\left( {{\mathbf{y}}_{E}}|{{x}_{2}} \right)}^{\text{H}}} \right\} =\left[ \begin{matrix}
   {{\left| {{g}_{1}} \right|}^{2}}{{\text{P}}_{1}}+\sigma _{E\text{,1}}^{2} & {{g}_{1}}{{\left( \mathbf{f}_{e}^{\text{T}}\mathbf{W}{{\mathbf{f}}_{1}} \right)}^{*}}{{\text{P}}_{1}}  \\
   g_{1}^{*}\left( \mathbf{f}_{e}^{\text{T}}\mathbf{W}{{\mathbf{f}}_{1}} \right){{\text{P}}_{1}} & {{\left| \mathbf{f}_{e}^{\text{T}}\mathbf{W}{{\mathbf{f}}_{1}} \right|}^{2}}{{\text{P}}_{1}}+\sigma_{R}^{2}||\mathbf{f}_{e}^{\text{T}}\mathbf{W}|{{|}^{2}}+\sigma_{E\text{,2}}^{2}\\
\end{matrix} \right].
\end{equation}}
\textcolor[rgb]{0,0.5,0}{Calculating the determinant of the above matrices and substituting into (\ref{AppII1}), one can arrive at the equation (\ref{botpage1}). By the same token, the equation (\ref{botpage2}) can be derived.}
